# Supplementary material for: Limits on Spectral Resolution Measurements by Quantum Probes
Source: arXiv:1707.01902 ancillary file (2019-02-17)
Supplement: Supplementary file 1 [file supplemental.pdf]

# Supplemental Material

## I. RESOLUTION LIMITS

In the following sections we analyze the resolving limits of different estimation methods. We start with a phase sensitive measurement with NV center. The dynamics of the NV center under DD is described by the Hamiltonian

$$\mathcal{H}(t) = \sigma_z \sum_k \Omega_k \sin(\delta_k t + \varphi_k), \tag{1}$$

where $\sigma_z$ refers to the $|0\rangle$ and $|1\rangle$ states of the NV, $\Omega$ is the Rabi-frequency of the signal, $\delta$ is the detuning of the signal from the DD frequency, $\varphi$ is the signal phase, and $k$ is an index for the different frequencies. The probability of measuring the NV in the $|\uparrow_y\rangle$ state, after initializing it in the $|\uparrow_x\rangle$, is given by

$$p_t = \sin^2\left(\phi(t) + \frac{\pi}{4}\right) \tag{2}$$

where

$$\phi(t) = \sum_{k=1}^{2} \Omega_k \tau \mathrm{sinc}\left(\frac{\delta_k \tau}{2}\right) \sin(\delta_k t + \varphi_k) \tag{3}$$

is the phase accumulated by the probe (i.e., half of the rotation angle over the Bloch sphere) during the measurement (in the time interval $\left(t - \frac{\tau}{2}, t + \frac{\tau}{2}\right)$), $\tau$ is the length of a single measurement (and is limited by the coherence time of the probe).

### A. Estimating frequencies out of the power spectrum

In this section we analyze the resolving power of estimating frequencies out of the power spectrum. In the limit of low detuning $\delta_k \tau \ll 1$ and low power $\sum_k \Omega_k \tau \ll 1$ the probability of a positive measurement (Eqs. 2,3) is simplified to

$$p_t \approx \frac{1}{2} + \sum_{k=1}^{2} \Omega_k \tau \sin(\delta_k t + \varphi_k).$$

The correlation function of measurement is thus given by

$$C_t = \frac{1}{4} + \frac{1}{2}\sum_{k=1}^{2} \Omega_k^2 \tau^2 \cos(\delta_k t) f_k(t),$$

with a noise that scales like $\sim \sqrt{\tau/T}$, where $f(t)$ is a decay function that depends on the type of noise, and $T$ is the total time of the measurement sequence. Here we analyze two types of noise, one that generates a Lorentzian line shape ($f(t) = e^{-t/T_\varphi}$), and another that generates a Gaussian line shape ($f(t) = e^{-(t/T_\varphi)^2}$), where $T_\varphi$ is the coherence time of the phase.

*Lorentzian line shape* The Lorentzian line shape is given by

$$S_\omega^{(L)} \sim \sum_{k=1}^{2} \frac{\Omega_k^2 \tau^2}{\left((\omega - \delta_k) T_{\varphi,k}\right)^2 + 1},$$

with noise that scales like $\sim \sqrt{\tau/T}$ (generally the noise is dependent on the frequency $\omega$, this will only give a numerical factor for the uncertainty). The regime in which it is difficult to resolve the frequencies is when the amplitudes and coherence times are equal. The Fisher-Information (FI) of $\delta_2 - \delta_1$ in this case is

$$I_{\delta_2-\delta_1} \sim \sum_\omega \frac{T}{\tau}\left(\frac{\mathrm{d}S(\omega)}{\mathrm{d}(\delta_2 - \delta_1)}\right)^2 \sim \Omega^4 \tau^3 T_\varphi^4 T (\delta_2 - \delta_1)^2.$$

Thus, the uncertainty (for both known and unknown $\Omega, T_\varphi$) is limited by the Cramér-Rao bound (CRB)

$$\Delta(\delta_2 - \delta_1) \sim \frac{1}{\Omega^2 \tau^{3/2} T_\varphi^2 \sqrt{T} (\delta_2 - \delta_1)}.$$

This means that if the beat-note frequency is smaller by a factor of 10, the time of the experiment should be extended by a factor of 100.

*Gaussian line-shape* The Gaussian line-shape is given by

$$S_{\omega}^{(G)} \sim \sum_{k=1}^{2} \Omega_k^2 \tau^2 \exp\left(-\left(\left(\omega-\delta_k\right) T_{\varphi,k}/2\right)^2\right),$$

with noise that scales like $\sim \sqrt{\tau/T}$. The regime in which it is difficult to resolve the frequencies is when the amplitudes and coherence times are equal. The FI of $\delta_2-\delta_1$ in this case is

$$I_{\delta_2-\delta_1} \sim \Omega^4 \tau^3 T_{\varphi}^4 T \left(\delta_2-\delta_1\right)^2,$$

as for the Lorentzian case. In the case that $\Omega, T_{\varphi}$ are unknown, inverting the full FI matrix will yield an uncertainty of

$$\Delta\left(\delta_2-\delta_1\right) \sim \frac{1}{\Omega^2 \tau^{3/2} T_{\varphi}^4 \sqrt{T}\left(\delta_2-\delta_1\right)^3}.$$

This means that if the beat-note frequency is smaller by a factor of 10, the time of the experiment should be extended by a factor of $10^6$ .

### B. Resolution limits for a coherent signal (phase sensitive measurement)

In the following we investigate the model in which all parameters are constant, except for the phases which undergo a certain random process with a time scale of $T_{\varphi}$. This is a good approximation to state of the art RF sources since the amplitude fluctuations are much smaller than the mean values. Therefore for periods shorter than $T_{\varphi}$ the phases can be considered constant. A long enough $T_{\varphi}$ allows us to make a large number of measurements in which the phases $\varphi_1, \varphi_2$ are constant. Note that the scenario in which the amplitudes also change in a random fashion is examined in section I C.

The phase sensitive measurement is described in Fig. 1b in the main text. A set of $n$ measurements is made during a period shorter than the coherence time of the signal (so that the phases are constant). Each measurement is performed as in a standard Ramsey experiment. The length of a single measurement is given by $\tau$, which is limited by the coherence time of the probe ($T_2$). The transition probability is given in Eqs. 2,3. It can be seen that the FI matrix due to this measurement at time $t$ is given by:

$$I_{i,j}^{(t)} = \frac{1}{p_t\left(1-p_t\right)} \frac{\mathrm{d}p_t}{\mathrm{d}\theta_i} \frac{\mathrm{d}p_t}{\mathrm{d}\theta_j} = 4 \frac{\mathrm{d}\phi\left(t\right)}{\mathrm{d}\theta_i} \frac{\mathrm{d}\phi\left(t\right)}{\mathrm{d}\theta_j}. \tag{4}$$

where $\theta_j$ stands for the unknown parameters we want to estimate. Each single measurement yields a FI matrix of this form, and since all measurements are independent, the total FI matrix is the sum of all these matrices.

We are now poised to make a detailed variance analysis. We aim to target the challenging regime of $|\delta_1-\delta_2|T \ll 1$, where $T$ is the total measurement time and is limited by the coherence time of the signal, and the stability of the clock.

#### 1. *Resolvable regime*

Let us first analyze the simpler case of $|\delta_1-\delta_2|T > 1$, in which the frequencies are assumed to be resolvable. For small $\delta_j\tau$, and large $\delta_j T$, the FI about $\delta_i$ is:

$$I_{\delta_j,\delta_j} \approx \sum_t 4\Omega_j^2 \tau^2 t^2 \cos\left(\delta_j t+\varphi_j\right)^2 \approx \frac{2}{3}\Omega_j^2 \tau T^3$$

and:

$$I_{\delta_1,\delta_2} \approx \sum_t 4\Omega_1\Omega_2 \tau^2 t^2 \cos\left(\delta_1 t+\varphi_1\right)\cos\left(\delta_2 t+\varphi_2\right) \approx 0$$

where the last approximation step is correct under our assumption that $|\delta_1+\delta_2|T,\ |\delta_1-\delta_2|T \gg 1$. Similarly, we can calculate all the other terms in the FI matrix, and obtain:

$$\begin{pmatrix} I_{\delta_1,\delta_1} & I_{\delta_1,\delta_2} & I_{\delta_1,\varphi_1} & I_{\delta_1,\varphi_2} & I_{\delta_1,\Omega_1} & I_{\delta_1,\Omega_2} \\ I_{\delta_2,\delta_1} & I_{\delta_2,\delta_2} & I_{\delta_2,\varphi_1} & I_{\delta_2,\varphi_2} & I_{\delta_2,\Omega_1} & I_{\delta_2,\Omega_2} \\ I_{\varphi_1,\delta_1} & I_{\varphi_1,\delta_2} & I_{\varphi_1,\varphi_1} & I_{\varphi_1,\varphi_2} & I_{\varphi_1,\Omega_1} & I_{\varphi_1,\Omega_2} \\ I_{\varphi_2,\delta_1} & I_{\varphi_2,\delta_2} & I_{\varphi_2,\varphi_1} & I_{\varphi_2,\varphi_2} & I_{\varphi_2,\Omega_1} & I_{\varphi_2,\Omega_2} \\ I_{\Omega_1,\delta_1} & I_{\Omega_1,\delta_2} & I_{\Omega_1,\varphi_1} & I_{\Omega_1,\varphi_2} & I_{\Omega_1,\Omega_1} & I_{\Omega_1,\Omega_2} \\ I_{\Omega_2,\delta_1} & I_{\Omega_2,\delta_2} & I_{\Omega_2,\varphi_1} & I_{\Omega_2,\varphi_2} & I_{\Omega_2,\Omega_1} & I_{\Omega_2,\Omega_2} \end{pmatrix} = 4 \begin{pmatrix} \Omega_1^2 T^3 \frac{\tau}{6} & 0 & \Omega_1^2 T^2 \frac{\tau}{4} & 0 & 0 & 0 \\ 0 & \Omega_2^2 T^3 \frac{\tau}{6} & 0 & \Omega_2^2 T^2 \frac{\tau}{4} & 0 & 0 \\ \Omega_1^2 T^2 \frac{\tau}{4} & 0 & \Omega_1^2 T \frac{\tau}{2} & 0 & 0 & 0 \\ 0 & \Omega_2^2 T^2 \frac{\tau}{4} & 0 & \Omega_2^2 T \frac{\tau}{2} & 0 & 0 \\ 0 & 0 & 0 & 0 & T\frac{\tau}{2} & 0 \\ 0 & 0 & 0 & 0 & 0 & T\frac{\tau}{2} \end{pmatrix}.$$

The CRB for the variance of $\delta_j$ is $\text{var}\left(\delta_j\right) \geq \left[I^{-1}\right]_{\delta_j,\delta_j}$, where $I^{-1}$ is the inverse of the FI matrix. Thus, for the matrix above, the only non-vanishing non-diagonal terms are $I_{\delta_j,\varphi_j}$ (these terms affect the CRB when taking the inverse of the FI matrix), which accounts for the small increase in the variance compared to the case in which all the other parameters except the frequencies are known (in this case the CRB is $\text{var}\left(\delta_j\right) \geq 1/I_{\delta_j,\delta_j}$): $\text{var}\left(\delta_j\right) = 6\left(\Omega_j^2 \tau T^3\right)^{-1}$, and $\text{var}\left(\delta_1 - \delta_2\right) = 6\left(\Omega_1^{-2} + \Omega_2^{-2}\right)\left(\tau T^3\right)^{-1}$.

### 2. *Unresolvable regime*

Let us now concentrate on the supposedly unresolvable regime; i.e., $|\delta_1 - \delta_2| T \ll 1$. It is easy to see that all the diagonal terms in the FI matrix do not change, whereas the non-diagonal terms do change, for example:

$$
\begin{aligned}
I_{\delta_1,\delta_2} =& \sum_t 4\Omega_1\Omega_2 t^2\tau^2 \cos\left(\delta_1 t + \varphi_1\right)\cos\left(\delta_2 t + \varphi_2\right) \approx \sum_t 2\Omega_1\Omega_2 t^2 \tau^2 \cos\left(\varphi_1 - \varphi_2\right) \\
\approx& \frac{2}{3}\Omega_1\Omega_2\tau T^3 \cos\left(\varphi_1 - \varphi_2\right).
\end{aligned}
$$

*Known amplitudes* We first consider the case in which the amplitudes $(\Omega_1, \Omega_2)$ are known, then the FI matrix in the limit of $\delta_1 - \delta_2 \to 0$ reads:

$$
\begin{pmatrix}
I_{\delta_1,\delta_1} & I_{\delta_1,\delta_2} & I_{\delta_1,\varphi_1} & I_{\delta_1,\varphi_2} \\
I_{\delta_2,\delta_1} & I_{\delta_2,\delta_2} & I_{\delta_2,\varphi_1} & I_{\delta_2,\varphi_2} \\
I_{\varphi_1,\delta_1} & I_{\varphi_1,\delta_2} & I_{\varphi_1,\varphi_1} & I_{\varphi_1,\varphi_2} \\
I_{\varphi_2,\delta_1} & I_{\varphi_2,\delta_2} & I_{\varphi_2,\varphi_1} & I_{\varphi_2,\varphi_2}
\end{pmatrix}
= 4
\begin{pmatrix}
\frac{\Omega_1^2 T^3 \tau}{6} & \Omega_1\Omega_2 \cos\left(\varphi_1 - \varphi_2\right)\frac{T^3\tau}{6} & \Omega_1^2\tau\frac{T^2}{4} & \Omega_1\Omega_2\tau\frac{T^2}{4}\cos\left(\varphi_1 - \varphi_2\right) \\
\Omega_1\Omega_2\cos\left(\varphi_1 - \varphi_2\right)\frac{T^3\tau}{6} & \frac{\Omega_2^2 T^3\tau}{6} & \Omega_1\Omega_2\tau\frac{T^2}{4}\cos\left(\varphi_1 - \varphi_2\right) & \Omega_2^2\tau\frac{T^2}{4} \\
\Omega_1^2\tau\frac{T^2}{4} & \Omega_1\Omega_2\tau\frac{T^2}{4}\cos\left(\varphi_1 - \varphi_2\right) & \Omega_1^2\tau\frac{T}{2} & \Omega_1\Omega_2\tau\frac{T}{2}\cos\left(\varphi_1 - \varphi_2\right) \\
\Omega_1\Omega_2\tau\frac{T^2}{4}\cos\left(\varphi_1 - \varphi_2\right) & \Omega_2^2\tau\frac{T^2}{4} & \Omega_1\Omega_2\tau\frac{T}{2}\cos\left(\varphi_1 - \varphi_2\right) & \Omega_2^2\tau\frac{T}{2}
\end{pmatrix}.
\tag{5}
$$

Thus there is a critical dependence on $\varphi_1 - \varphi_2$. In general the variance of $\delta_1 - \delta_2$ is:

$$
\text{var}\left(\delta_1 - \delta_2\right) = 24\left(\Omega_1^{-2} + \Omega_2^{-2}\right)\left(\tau T^3\right)^{-1} \cdot \frac{1 - \frac{2\Omega_1\Omega_2}{\Omega_1^2 + \Omega_2^2}\cos\left(\varphi_1 - \varphi_2\right)}{\sin^2\left(\varphi_1 - \varphi_2\right)},
$$

hence we get an infinite variance when $\varphi_1 - \varphi_2 = 0, \pi$ and $\Omega_1 \neq \Omega_2$ (or $\varphi_1 - \varphi_2 = 0$ and $\Omega_1 = \Omega_2$) . It is noteworthy that this case corresponds to the hyper-polarized case in nano NMR in which the phase of the two signals is equal because of the polarization. This shows that in the unresolvable DFT case the statistical polarized signal contains more information in the case of similar signal strengths. It is interesting to see that while polarization increases the resolution decreases.

*Unknown amplitudes* When also including unknown amplitudes, we get the following FI matrix: in the limit of $\delta_1 - \delta_2 \to 0$,

$$
4
\begin{pmatrix}
\frac{\Omega_1^2 T^3\tau}{6} & \Omega_1\Omega_2\cos\left(\varphi_1 - \varphi_2\right)\frac{T^3\tau}{6} & \Omega_1^2\tau\frac{T^2}{4} & \Omega_1\Omega_2\tau\frac{T^2}{4}\cos\left(\varphi_1 - \varphi_2\right) & 0 & \Omega_1\tau\sin\left(\varphi_2 - \varphi_1\right)\frac{T^2}{4} \\
\Omega_1\Omega_2\cos\left(\varphi_1 - \varphi_2\right)\frac{T^3\tau}{6} & \frac{\Omega_2^2 T^3\tau}{6} & \Omega_1\Omega_2\tau\frac{T^2}{4}\cos\left(\varphi_1 - \varphi_2\right) & \Omega_2^2\tau\frac{T^2}{4} & \Omega_2\tau\sin\left(\varphi_1 - \varphi_2\right)\frac{T^2}{4} & 0 \\
\Omega_1^2\tau\frac{T^2}{4} & \Omega_1\Omega_2\tau\frac{T^2}{4}\cos\left(\varphi_1 - \varphi_2\right) & \Omega_1^2\tau\frac{T}{2} & \Omega_1\Omega_2\tau\frac{T}{2}\cos\left(\varphi_1 - \varphi_2\right) & 0 & \Omega_1\tau\sin\left(\varphi_2 - \varphi_1\right)\frac{T}{2} \\
\Omega_1\Omega_2\tau\frac{T^2}{4}\cos\left(\varphi_1 - \varphi_2\right) & \Omega_2^2\tau\frac{T^2}{4} & \Omega_1\Omega_2\tau\frac{T}{2}\cos\left(\varphi_1 - \varphi_2\right) & \Omega_2^2\tau\frac{T}{2} & \Omega_2\tau\sin\left(\varphi_1 - \varphi_2\right)\frac{T}{2} & 0 \\
0 & \Omega_2\tau\sin\left(\varphi_1 - \varphi_2\right)\frac{T^2}{4} & 0 & \Omega_2\tau\sin\left(\varphi_1 - \varphi_2\right)\frac{T}{2} & \frac{T}{2}\tau & \cos\left(\varphi_1 - \varphi_2\right)\tau\frac{T}{2} \\
\Omega_1\tau\sin\left(\varphi_2 - \varphi_1\right)\frac{T^2}{4} & 0 & \Omega_1\tau\sin\left(\varphi_2 - \varphi_1\right)\frac{T}{2} & 0 & \cos\left(\varphi_1 - \varphi_2\right)\tau\frac{T}{2} & \frac{T}{2}\tau
\end{pmatrix}.
$$

It can be shown that this matrix is singular for any values of $\Omega_1, \Omega_2$, and that the null space is spanned by the following vectors:

$$
\begin{gathered}
\left(0, 0, 0, -\sin\left(\varphi_2 - \varphi_1\right), \Omega_2, -\Omega_2\cos\left(\varphi_2 - \varphi_1\right)\right) \\
\left(0, 0, -\sin\left(\varphi_2 - \varphi_1\right), 0, -\Omega_1\cos\left(\varphi_1 - \varphi_2\right), \Omega_1\right).
\end{gathered}
$$

To get a better understanding of this behavior, note that the accumulated phase (Eq. 3) during the measurement at time $t$, when $|\delta_2 - \delta_1| T_\varphi \ll 1$, reads:

$$
\phi\left(t\right) \approx a\sin\left(\delta t + \alpha\right) + \frac{1}{2}b\Delta\delta t\cos\left(\delta t + \beta\right),
\tag{6}
$$

where $\Delta\delta = \delta_2 - \delta_1$, $\delta = \frac{\delta_2 + \delta_1}{2}$, and

$$
\begin{aligned}
a\sin\left(\delta t + \alpha\right) &= \left(\Omega_1\tau\sin\left(\delta t + \varphi_1\right) + \Omega_2\tau\sin\left(\delta t + \varphi_2\right)\right)\text{sinc}\left(\frac{\delta\tau}{2}\right) \\
b\cos\left(\delta t + \beta\right) &= \left(\Omega_1\tau\cos\left(\delta t + \varphi_1\right) - \Omega_2\tau\cos\left(\delta t + \varphi_2\right)\right)\text{sinc}\left(\frac{\delta\tau}{2}\right).
\end{aligned}
$$

Therefore, for a small beat-note the probability depends solely on $a, \alpha, b\Delta\delta, \beta$, which means that it is impossible to get information on $\Delta\delta, \Omega_1, \Omega_2, \varphi_1, \varphi_2$ separately. This indeed means that the FI matrix is singular.

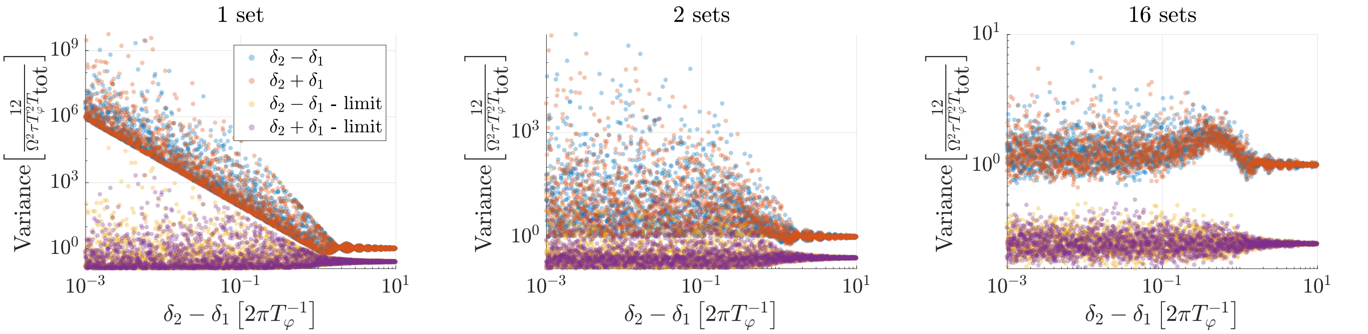


(a) (b) (c)

Figure 1. The Cramér-Rao bound for the variance of $\delta_2 \pm \delta_1$ is plotted as a function of $(\delta_2 - \delta_1) T_\varphi$ - normalized to the variance in the $(\delta_2 - \delta_1) T_\varphi \gg 1$ regime; i.e., $12/\left(\Omega^2 \tau T_\varphi^2 T_{tot}\right)$, calculated from the probability $x \sim B\left(\frac{1}{2} + \frac{1}{2}\sin\left(2\sum_{j=1}^{2}\Omega_j \tau \operatorname{sinc}(\delta_j \tau/2)\cos(\delta_j t + \varphi_j)\right)\right)$ while assuming unknown frequencies, amplitudes, and multiple sets of phases. The Cramér-Rao bound is dependent on the specific phases used; hence, the random phases generate a variance of the Cramér-Rao bound which decreases as more phases are included. For a single dataset ($6 \times 6$ covariance matrix) the $\left((\delta_2 - \delta_1) T_\varphi\right)^{-2}$ divergence is clearly shown (Fig. a), with only two datasets ($8 \times 8$ covariance matrix) this divergence is averted (Fig. b), nevertheless, the probability for error is large. With 16 datasets ($36 \times 36$ covariance matrix) the variance is comparable to the $(\delta_2 - \delta_1) T_\varphi \gg 1$ regime. $\delta, \Omega$ are given in Hz. the 'limit' refers to the Cramér-Rao bound when all other parameters are known. Note that the divergence of $\Delta(\delta_2 \pm \delta_1)$ comes from degeneracy, and the likelihood function still has a finite width on the order of $1/T_\varphi$.

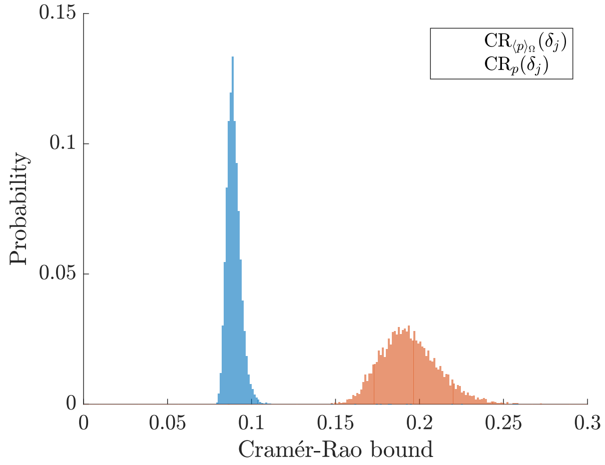


Figure 2. The Cramér-Rao bound for the uncertainty of $\delta_k$ for the parameter range of the experimental data (Sec. *experimental results* in the main text). In blue is the bound when assuming that all 33 amplitudes are the same; i.e., coming from a delta distribution. In red is the bound when trying to estimate all 33 amplitudes. The spread of the bound is due to random phases.

### 3. *Random phases*

It is possible to get rid of this divergence by including more phases in a random way; i.e., by taking multiple measurements - each with different phases - thus breaking the degeneracy and getting rid of the null space. Practically this means calculating the covariance from a $(2K + 4) \times (2K + 4)$ FI matrix (4 for the frequencies and amplitudes and $K$ pairs of phases). Intuitively we can approximate the FI matrix by assuming that the information about each set of $K$ phases is actually information about the same phase. Thus, by summing the FI matrix from all $K$ matrices most of the non-diagonal terms in the FI matrix are averaged to zero. After averaging, the FI matrix in the unresolvable regime takes on a similar structure as the FI in the resolvable regime. The numerical results in Fig. 1 show that the FI with multiple phases is comparable to the FI when the amplitudes are known.

### 4. Short coherence time

Recall that in a standard phase sensitive measurement experiment, the number of measurements in each coherent sequence, denoted $n$, is very large, namely $n \gg 1$. This is the case when the coherence time of the signal is much longer than the coherence time of the probe. What happens when the coherence time of the signal is much shorter so that only a few measurements can be performed in each sequence? This is the case of $n = \mathcal{O}(1)$. Since the FI about $\delta_1, \delta_2$ goes as $n^3$, the small $n$ implies much worse FI. Qualitatively, the behavior is quite similar to that of standard phase-sensitive measurement. The main limitation here is the requirement that $\delta_1 T_\varphi, \delta_2 T_\varphi$ must not be much smaller than one, where $T_\varphi$ is the length of a single sequence, since in that case the FI matrix becomes singular. This is illustrated in Fig. 3 which shows that the variance of $\delta_1, \delta_2$ converges to the optimal value, once $(\delta_1 + \delta_2) T_\varphi$ is large enough.

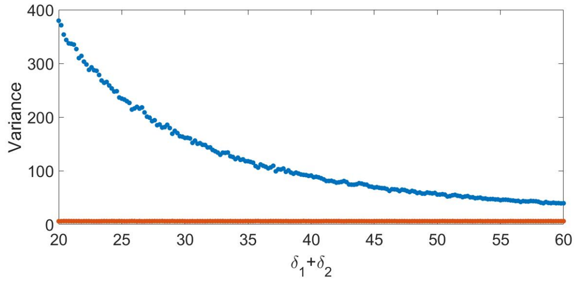


Figure 3. Variance of $\delta_1$ as a function of $\delta_1 + \delta_2$ for the case where number of measurements in each coherent sequence is 10.

### 5. Numerical results

We simulated the case of phase sensitive measurement, where we initialize the NV to state $|\uparrow_x\rangle$ and the probability for ending in state $|\uparrow_y\rangle$ is given by $p_j = \frac{1}{2} + \frac{1}{2}\sin\left(2\sum_{k=1}^{2}\Omega_k \tau \mathrm{sinc}\left(\frac{\delta_k \tau}{2}\right)\sin\left(\delta_k t_j + \varphi_k\right)\right)$. The probability of detecting a photon at the j'th measurement is $q_j = r_{\downarrow_y}(1-p_j) + r_{\uparrow_y} p_j$, where $r_{\downarrow_y}$ and $r_{\uparrow_y}$ are the probabilities to detect a photon in the case that the NV is in the state $\downarrow_y$,$\uparrow_y$, respectively. This model is used to simulate the NV center case [1].

In order to show that we can resolve two frequencies with $|\delta_2 - \delta_1| < 2\pi T^{-1}$, we compared two scenarios: data with two frequencies with $\delta_2 - \delta_1 = 0.1 \times 2\pi T^{-1}$ (where $\delta_2 - \delta_1 >$ single frequency uncertainty $\Delta(\delta_{1,2}) \propto \left(\Omega\sqrt{\tau}T^{3/2}\sqrt{N}\right)^{-1}$). The numerical results are shown in Fig. 4b, and for comparison, data with a single frequency are shown in Fig. 4c. For both, we ran the MLE scheme, and searched for two frequencies. For the former, in each dataset we were able to separate the two frequencies by more than three $\Delta(\delta_{1,2})$, and for the latter, we saw separation of less than one $\Delta(\delta_1 - \delta_2)$ and statistics fitting to the half-normal-distribution, where the estimated standard deviation was calculated from the statistics, and could be estimated from FI. The deduction is that the data contain two frequencies and we can resolve them. This shows that the algorithm is able to differentiate between a single frequency signal and a signal with two frequencies.

## C. Random amplitudes

### 1. Problem

We now consider the case in which the amplitudes change randomly, so that only for a time slot shorter than the coherence time ($T_\varphi$) of the signal the phases and the amplitudes are approximately constant. In the limit of a small beat-note $|\delta_2 - \delta_1| T_\varphi \ll 1$, the accumulated phase (Eq. 3) during the measurement is reduced to Eq. 6. We further simplify this analysis by assuming we have perfect knowledge of the main frequency, and setting it to zero. Thus, Eq. 6 reduces to

$$\phi(t) \approx x + 0.5 y \Delta\delta t, \tag{7}$$

where $x = a\sin\alpha$, $y = b\cos\beta$, and both are normally distributed around zero with variance $\sigma_y \sim \Omega\tau$. From a single set of correlated measurements we can only estimate $x$, and $y\Delta\delta$. The likelihood function for $y\Delta\delta$ given the estimation $e_j$ is given by

$$L_j(y\Delta\delta | e_j) \sim \exp\left(\frac{(y\Delta\delta - e_j)^2}{2\sigma^2}\right),$$

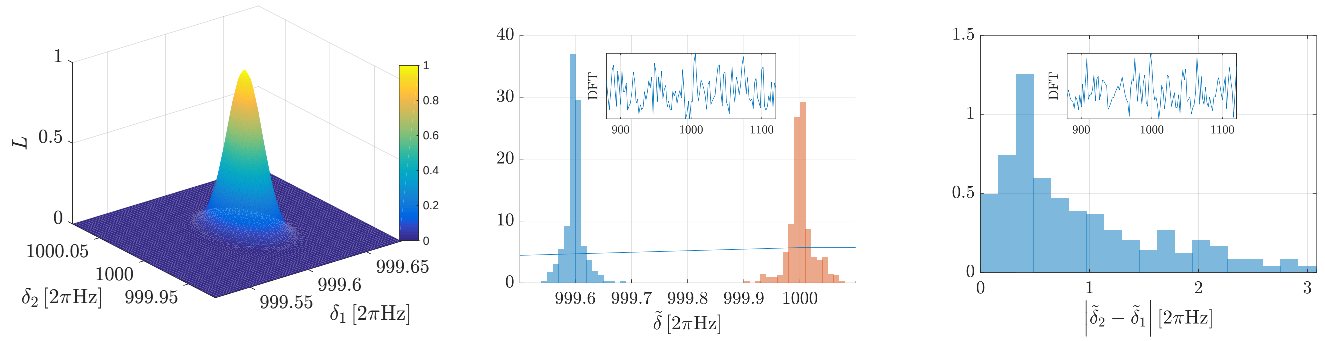


Figure 4. *Numerical results* (a) A typical likelihood function as a function of the frequency estimators $\delta_1$ and $\delta_2$ while keeping the other parameters fixed $(\Omega_k, \phi_k)$. In this analysis the real frequencies are $\delta_1 = 999.6[2\pi\text{Hz}]$ and $\delta_2 = 1000[2\pi\text{Hz}]$, Rabi of $\Omega_1 = 1\text{MHz}, \Omega_2 = 0.7\text{MHz}$, and $25,000$ measurements were performed in a total time of $0.25\,[\text{sec}]$, which corresponds to a Discrete Fourier Transform (DFT) resolution of $T^{-1} = 4[\text{Hz}]$. The average detection efficiency was set to $0.1$ with a contrast of $70\%$. (b) Histogram of the estimators, $\tilde{\delta}_1$ and $\tilde{\delta}_2$, over 400 realizations. This means that for every single dataset the signal was resolved. The data were created with the same parameters as in (b). The inset, and the blue line over the histogram, show the DFT for a single dataset where the signal is unresolved. (c) Histogram of $|\tilde{\delta}_1 - \tilde{\delta}_2|$ for estimators, over 300 realizations, calculated from data with only a single frequency $\delta = 1000[2\pi\text{Hz}]$. The data are consistent with a Folded-Normal-Distribution; in other words the standard deviation is much larger than the mean; thus we cannot resolve two frequencies and conclude that there is only one frequency in the signal.

where $\sigma^2$ is the variance of the measurement and scales as $\sim \tau/T_\varphi^3$. Using our prior for $y$, the marginal for the beat-note is given by

$$L_j\left(\Delta\delta|e_j\right) \sim \frac{1}{\sqrt{\sigma^2 + \sigma_y^2\Delta\delta^2}} \exp\left(-\frac{e_j^2}{2\left(\sigma^2 + \sigma_y^2\Delta\delta^2\right)}\right).$$

The likelihood for the beat-note, after repeating this estimation procedure with $n$ realizations of $x, y$, is given by

$$\mathcal{L}\left(\Delta\delta|\{e_j\}\right) \sim \left(\sigma^2 + \sigma_y^2\Delta\delta^2\right)^{-n/2} \exp\left(-\frac{n\left(\sigma^2 + \sigma_y^2\Delta\delta_r^2\right)}{2\left(\sigma^2 + \sigma_y^2\Delta\delta^2\right)}\right),$$

where we substitute $\frac{1}{n}\sum_{j=1}^{n} e_j^2$ for $\sigma^2 + \sigma_y^2\Delta\delta_r^2$ - the sample variance, and $\Delta\delta_r$ is the real beat-note frequency. For small $\frac{\Delta\delta_r\sigma_y}{\sigma}$; i.e., $\Delta\delta \ll \frac{1}{\Omega\sqrt{\tau}T_\varphi^{3/2}}$, the width of this function scales as $n^{-1/4}$; i.e., in the case that the beat-note is smaller by a factor of 10 the total experiment time should be prolonged by a large factor of $10^4$. We claim that it is possible to obtain a better scaling by averaging the probability over the signal amplitude, as we show in the next section.

### 2. *Solution*

In the case of random amplitudes we suggest that instead of estimating all the different amplitudes (in each set of measurements different amplitudes should appear, just like with the phases) it would be preferable to make estimation according to the average probability; i.e., the probability averaged over the different possible values of amplitudes (given that the distribution of the amplitudes is known). As an example, let us consider the case in which the amplitudes $\Omega_1$ $(\Omega_2)$ are drawn from a Rayleigh distribution $R\left(\sqrt{\frac{2}{\pi}}\langle\Omega_1\rangle\right)$ $\left(R\left(\sqrt{\frac{2}{\pi}}\langle\Omega_2\rangle\right)\right)$, and the phases are uniformly distributed (assuming no correlation), which corresponds to the case where the signal originates from an unpolarized material, with a mean polarization of zero and a statistical polarization $\sim \Omega_{1,2}$. The average transition probability is given by averaging the probability in Eq. 2,3 according to the relevant distribution:

$$p_{av} = \frac{\pi^2}{4\langle\Omega_1\rangle^2\langle\Omega_2\rangle^2}\int p_t\Omega_1\Omega_2 \exp\left(-\frac{\pi}{4}\left(\frac{\Omega_1^2}{\langle\Omega_1\rangle^2} + \frac{\Omega_2^2}{\langle\Omega_2\rangle^2}\right)\right) \mathrm{d}\Omega_1\,\mathrm{d}\Omega_2. \tag{8}$$

Denoting $\phi_k = \langle\Omega_k\rangle\,\tau\text{sinc}\left(\frac{\delta_k\tau}{2}\right)\cos\left(\delta_k t + \varphi_k\right), (k = 1, 2)$, we get that the averaged probability reads:

$$p_{av} = \frac{1}{2} + \left(\phi_1 + \phi_2\right)\exp\left(-\frac{4}{\pi}\left(\phi_1^2 + \phi_2^2\right)\right). \tag{9}$$

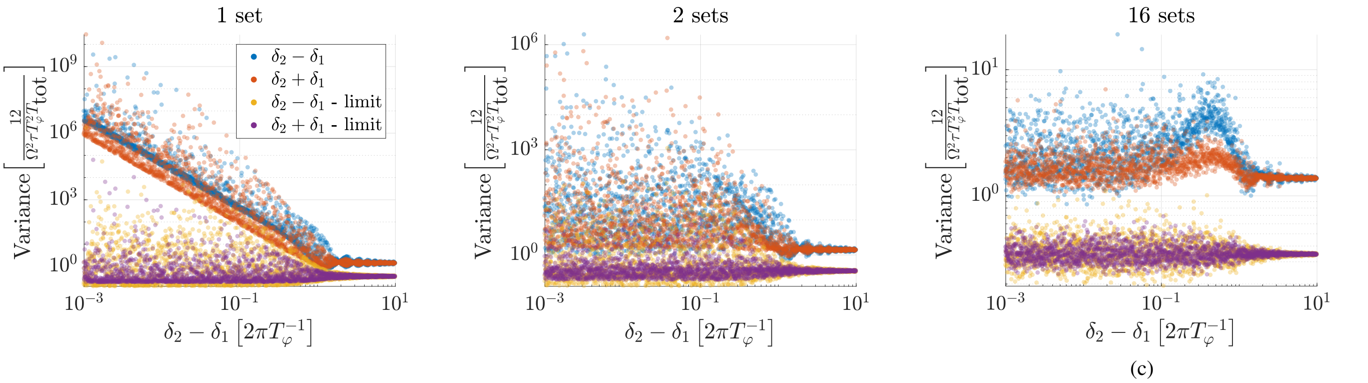


Figure 5. The Cramér-Rao bound for the variance of $\delta_2 \pm \delta_1$ is plotted as a function of $(\delta_2-\delta_1)\,T_\varphi$ - normalized to the variance in $(\delta_2-\delta_1)\,T_\varphi \gg 1$ regime $\left(12/\left(\langle\Omega\rangle^2 \tau T_\varphi^2 T_{tot}\right)\right)$, calculated from the average probability over amplitudes taken from a Rayleigh distribution $x \sim B\left(\frac{1}{2}+\alpha_t \exp\left[-\alpha_t^2 4/\pi\right]\right)$, where $\alpha_t = \sum_{j=1}^{2} \langle\Omega_j\rangle \tau \text{sinc}\,(\delta_j\tau/2)\cos(\delta_j t+\varphi_j)$, and while assuming unknown frequencies, averaged amplitudes, and multiple sets of phases. For a single dataset ($6\times6$ covariance matrix) the $\left((\delta_2-\delta_1)\,T_\varphi\right)^{-2}$ divergence is clearly shown (Fig. a), with only two datasets ($8\times8$ covariance matrix) this divergence is averted (Fig. b); nevertheless, the probability for error is large. With 16 datasets ($36\times36$ covariance matrix) the variance is comparable to the $(\delta_2-\delta_1)\,T_\varphi \gg 1$ regime. $\delta,\Omega$ are given in Hz. the 'limit' refers to the Cramér-Rao bound where all other parameters are known.

So the elements of the FI matrix now read:

$$I_{ij} = \frac{1}{p\,(1-p)}\frac{\mathrm{d}p_{av}}{\mathrm{d}\theta_i}\frac{\mathrm{d}p_{av}}{\mathrm{d}\theta_j} \tag{10}$$

For small amplitudes $\langle\Omega_k\rangle\tau \ll 1$, these elements can be simplified to $I_{ij} \approx 4\frac{d\phi_k}{d\theta_i}\frac{d\phi_l}{d\theta_j}$, which is similar to the FI matrix obtained with constant amplitudes (see Eq. 4). The behavior in this case appears to be very similar to the one observed with constant amplitudes (Fig. 1, Sec. I B 3), and thus there is no divergence of the variance for $|\delta_1-\delta_2|T \ll 1$ (Fig. 5). For large amplitudes $\langle\Omega_k\rangle\tau \gg 1$, the probability function becomes mostly flat with sharp peaks when $\phi_1^2+\phi_2^2 \approx 0$. Thus the FI goes to zero for any $\delta_k$.

## II. MAXIMUM-LIKELIHOOD ANALYSIS FOR PHASE SENSITIVE MEASUREMENT

We now consider the Maximum-Likelihood (ML) analysis performed in the coherent case. In order to distinguish between two close frequencies, beyond the resolution limit given by the discrete Fourier transform (DFT) $T^{-1}$, we would like to use multiple sets of measurements, with times $T$, and implement them to differentiate between two frequencies with $\Delta\delta < 2\pi T^{-1}$, using Maximum-Likelihood Estimation (MLE).

From the Hamiltonian in Eq. 1 we derive the transition probability (Eq. 11) form state $|\uparrow_x\rangle$ to state $|\uparrow_y\rangle$ after time $\tau$.

$$p_j = \sin^2\left(\sum_{k=1}^{2}\Omega_k\tau\text{sinc}\left(\frac{\delta_k\tau}{2}\right)\cos\left(\delta_k t_j+\varphi_k\right)+\frac{\pi}{4}\right) \tag{11}$$

where $\Omega_k$ is the Rabi frequency, and $\delta_k$ is the frequency. For the NV center case, the probability of detecting a photon is $q_j = r_\downarrow(1-p_j)+r_\uparrow p_j$, where $r_\uparrow$ ($r_\downarrow$) is the probability of detecting a photon from the up (down) state. We measure $n$ times from $t=0$ to $t=T$ and get the outcome vector $x$ ($x_j \in \{0,1\}$) at times $t_j = j\tau = j\frac{T}{n}$. In order to differentiate between two frequencies with $\Delta\delta = |\delta_2-\delta_1| < 2\pi T^{-1}$, we calculate the likelihood for outcome vector $x$,

$$L\left(x;t\,\middle|\,\{\Omega_k,\delta_k,\varphi_k\}_{k=1}^{2}\right) = \prod_{j=1}^{n} q_j^{x_j}\left(1-q_j\right)^{1-x_j}.$$

Finding the maximum point of the likelihood function gives the estimators, $\tilde{\Omega}_k, \tilde{\delta}_k, \tilde{\varphi}_k$ (for now, we only care about $\tilde{\delta}_k$).

Given multiple sets of coherent measurements (each of time $T$), where for each realization, $\Omega_k, \delta_k$ remain constant, and the phase $\varphi_k$ is random. The likelihood for each outcome vector $x^{(\ell)}$ is

$$L_\ell = L\left(x^{(\ell)};t\,\middle|\left\{\tilde{\Omega}_k,\tilde{\delta}_k,\tilde{\varphi}_k^{(\ell)}\right\}_{k=1}^{2}\right).$$

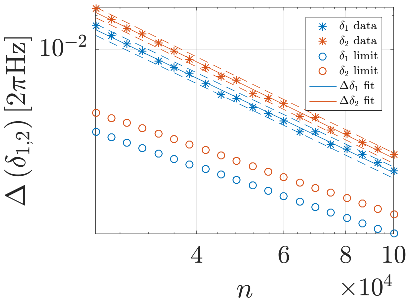


(a)

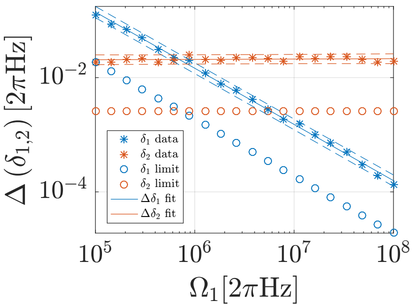


(b)

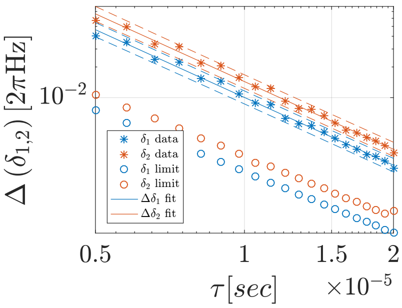


(c)

Figure 6. *Scaling analysis* (a) Scaling as a function of the number of measurements. The standard deviation of the estimators $\tilde{\delta}_1, \tilde{\delta}_2$, shown as $*$, as a function of the number of measurements ($\propto T$). For reference, the Cramér-Rao bound is shown as $\circ$ for the two frequencies. The dashed lines correspond to a width of two standard deviations of the fit. The logarithmic fit gives a power of $2.12 \pm 0.06$, compared to $^3/_2$ for the single frequency estimation (Eq. 12). The discrepancy between the two is due to the fact that the Cramér-Rao bound is not saturated and the two should overlap for larger $n$. (b) Scaling as a function of the Rabi Frequency. The Rabi frequency of one of the signals was changed and a scaling of $0.98 \pm 0.02$ was verified, compared to 1 for a single frequency (Eq. 12). (c) Scaling as a function of measurement time. The time of each run ($\tau$) was changed and a scaling power of $2.21 \pm 0.08$ was verified, compared to 2 for the Cramér-Rao bound (Eq. 12).

Thus the complete Likelihood function is

$$\mathcal{L} = \prod_{\ell=1}^{N} L_\ell,$$

where $N$ is the number of uncorrelated measurement sets. The values of $\delta_k$ that maximize the likelihood function are chosen to be the estimated values of the frequencies that we wish to find. Using FI we derived the CRB for the Standard deviation of the estimator

$$\Delta(\delta_n) = \sqrt{12}\sqrt{\frac{\frac{r_\uparrow + r_\downarrow}{2}\left(1 - \frac{r_\uparrow + r_\downarrow}{2}\right)}{\left(r_\uparrow - r_\downarrow\right)^2}}\frac{1}{\Omega_n\sqrt{\tau}T_\varphi^{3/2}\sqrt{N}} \tag{12}$$

Eq. 12 implies that with enough measurement sets, we can break the DFT limit of $T^{-1}$.

### A. Scaling analysis

To verify the validity of Eq. 12 for resolution we ran the MLE scheme for a range of parameters and fitted the estimated standard deviation to the CRB. The results are presented in Fig. 6. In all the figures the standard deviation approaches the bound and is expected to saturate the bound with a larger number of measurements. The FI depends on the way that the data are analyzed; thus Eq. 12 was modified, see section I B. The analysis here is shown for a large number of measurements. However, the conclusion that precision and resolution are very closely connected is also valid for a smaller number of measurements.

### B. Numerics for signals with a short coherence time

For signals with short coherence time compared with the probe coherence time; i.e., where it is not possible to perform multiple measurements to properly estimate the phase, it is still beneficial to perform multiple measurements at the cost of shortening them below the coherence time of the probe. Doing so provides information about the signal phase for each dataset, and thus makes it possible to estimate the frequencies. In Fig. 7 we show that we can resolve two frequencies with a difference of $0.05 \times T^{-1}$, by using 30 sets of data, each containing 10 coherent measurements.

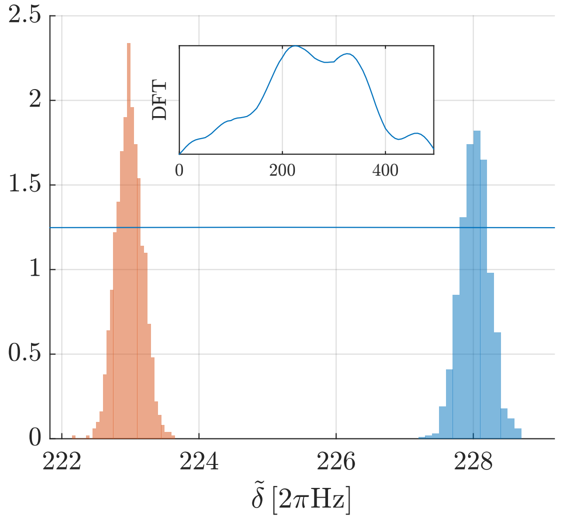


Figure 7. Histogram of the estimators $\tilde{\delta}_1$ and $\tilde{\delta}_2$ from the MLE, over $1,000$ realizations. The data were created with two signals $\delta_1 = 228\,[2\pi\text{Hz}]$ and $\delta_2 T = 223\,[2\pi\text{Hz}]$, with power $\Omega_1 = 2\,[2\pi\text{kHz}]$ and $\Omega_2 = 2.3\,[2\pi\text{kHz}]$, measured $n = 10$ times for each coherent dataset of time $T = 0.01\,[\text{sec}]$, and $N = 30$ datasets were generated. The average estimators from the MLE are $\left\langle \tilde{\delta}_1 \right\rangle 223.0 \pm 0.2\,[2\pi\text{Hz}]$, and $\left\langle \tilde{\delta}_2 \right\rangle 228.0 \pm 0.2\,[2\pi\text{Hz}]$. The inset, and the blue curve over the histogram, show the average DFT over the entire data.

### C. Numerics for data with multiple frequencies

As the experiment involved extra frequencies which are multiplets of 100Hz, we analyzed this case numerically to estimate the effect of these frequencies on the MLE results. In order to show how a general spectrum influences the MLE, we conducted two analyses with similar data only differing by the extra spectral noise at $\delta$ equals 100, 200, and 300 $[2\pi\text{Hz}]$ (Fig. 8). The result in Fig. 8 shows that other frequencies in the spectra can affect the variance of the estimators. This effect can be compensated for including extra frequencies in the numerical analysis.

### D. multiple frequencies

We tentatively explored the possibility of generalizing the analysis to a signal containing multiple unknown frequencies. Fig. 9 shows the MLE analysis for a signal containing three close frequencies at 250, 251.5 and 253 [$2\pi$ Hz]. The results show that the problem of resolving a multi-frequency signal is not conceptually different from a two-frequency signal; it just requires more computation time. The simulation effort can be solved employing parallelization techniques for the different samples for which we need to generate the statistics.

## III. CORRELATION BETWEEN THE PHASES

We analyzed a simple dephasing model in which there exists a fixed correlation time after which the phases are uncorrelated. In a more realistic scenario some correlation exists which is characterized by a probability of $\varphi_i$ given $\varphi_{i-1}$: $p(\varphi_i|\varphi_{i-1})$. In this case the calculation is be done in the following way. By Bayes' rule we get:

$$p(\delta,\varphi_1,\varphi_2,...,\varphi_n|\{x_i\}) \propto p(\{x_i\}|\delta,\varphi_1,\varphi_2,...,\varphi_n)p(\delta,\varphi_1,\varphi_2,...,\varphi_n), \tag{13}$$

where $x_i$ are the measurement results and

$$p(\delta,\varphi_1,\varphi_2,...,\varphi_n) = p(\delta)p(\varphi_1)p(\varphi_2|\varphi_1)p(\varphi_3|\varphi_2)...p(\varphi_n|\varphi_{n-1}). \tag{14}$$

As $p(\delta)$ has a uniform distribution we will get:

$$\begin{aligned} p(\delta,\varphi_1,\varphi_2,...,\varphi_n|\{x_i\}) &\propto p(\{x_i\}|\delta,\varphi_1,\varphi_2,...,\varphi_n)p(\varphi_1)p(\varphi_2|\varphi_1)p(\varphi_3|\varphi_2)...p(\varphi_n|\varphi_{n-1}) \\ &= p(x_1|\delta,\varphi_1)p(x_2|\delta,\varphi_2)...p(x_n|\delta,\varphi_n)p(\varphi_1)p(\varphi_2|\varphi_1)p(\varphi_3|\varphi_2)...p(\varphi_n|\varphi_{n-1}) \end{aligned} \tag{15}$$

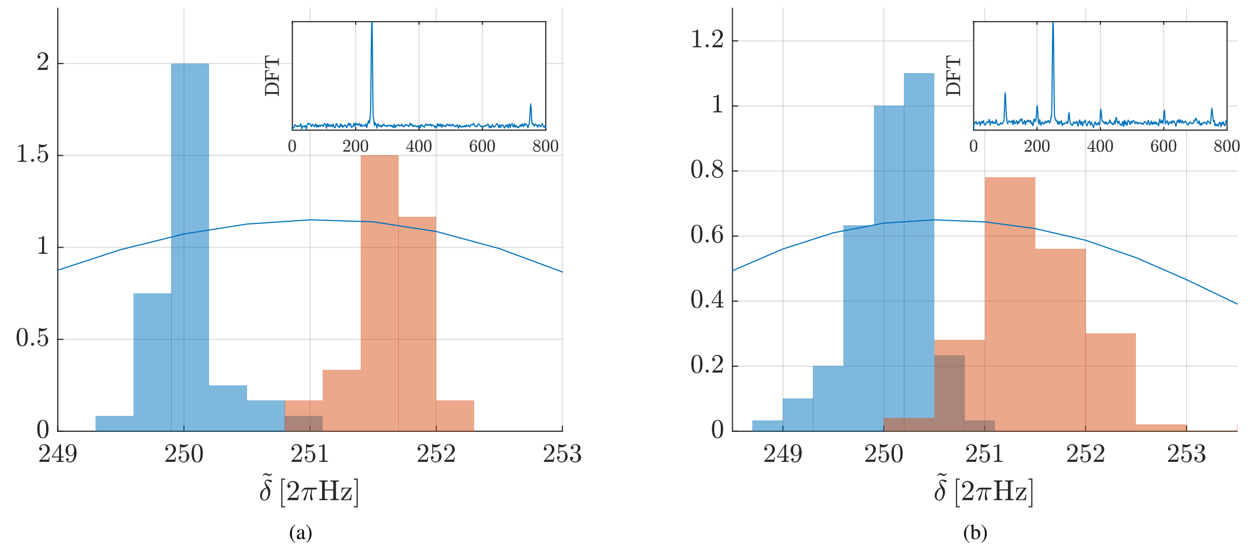


Figure 8. Histogram of the estimators $\tilde{\delta}_1$ and $\tilde{\delta}_2$ from the MLE over 200 realizations. The inset, and the blue curve over the histogram show the average DFT over the entire data. The data were created with two signals $\delta_1 = 250$ [$2\pi$Hz] and $\delta_2 = 251.6$ [$2\pi$Hz], with a Rabi-frequency $\Omega \approx 12$ [$2\pi$kHz], measured $n = 25,000$ times for each coherent dataset of time $T = 0.25$ [sec], and $N = 4$ datasets were generated. (a) The data were generated with no extra signals (see inset), and the MLE results in $\left\langle \tilde{\delta}_1 \right\rangle = 250.1 \pm 0.3$ [$2\pi$Hz], and $\left\langle \tilde{\delta}_2 \right\rangle = 251.6 \pm 0.3$ [$2\pi$Hz] . (b) The data were generated with extra signals of $\delta$ equals 100, 200, and 300 [$2\pi$Hz] (see inset), and the MLE results in $\left\langle \tilde{\delta}_1 \right\rangle = 250.1 \pm 0.4$ [$2\pi$Hz], and $\left\langle \tilde{\delta}_2 \right\rangle = 251.5 \pm 0.6$ [$2\pi$Hz].

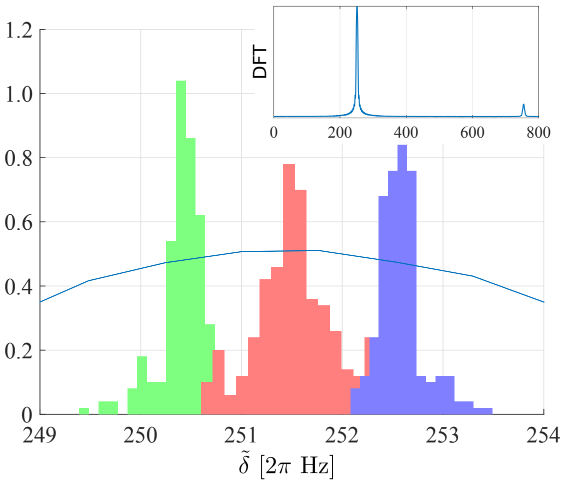


Figure 9. Histogram of the estimators $\tilde{\delta}_1$, $\tilde{\delta}_2$ and $\tilde{\delta}_3$ from the MLE over 200 realizations. The inset, and the blue curve over the histogram show the average DFT over the entire data. The data were created with three signals $\delta_1 = 250.0$ [$2\pi$Hz], $\delta_2 T = 251.5$ [$2\pi$Hz] and $\delta_2 T = 253.0$ [$2\pi$Hz], with power $\Omega_1 = 10$ [$2\pi$kHz], $\Omega_2 = 11$ [$2\pi$kHz] and $\Omega_3 = 12$ [$2\pi$kHz], measured $n = 2^{15}$ times for each coherent dataset of time $T = 0.32$ [sec], and $N = 64$ datasets were generated.

We know how to calculate all these terms. For example in the case of diffusion noise $p(\varphi_2|\varphi_1) = \exp\left[-\frac{(\varphi_1-\varphi_2)^2}{2\sigma^2}\right]/\sqrt{2\pi\sigma^2}$ and thus the coherence time ($T_\varphi = 2\tau/\sigma^2$) becomes an extra parameter that can be estimated by MLE. It is noteworthy that this distribution is unbounded and thus should be discretized in the ML procedure [2].

## IV. EXPERIMENTAL PROCEDURE

All experiments were performed on a single NV center, approximately 3 $\mu$m below the surface of an ultrapure diamond with 99.999% $^{12}$C content. Read-out of the NV center was performed with a custom-built confocal microscope using a 500 ns duration laser pulse at 532 nm and 1.4 N.A. oil objective. This same laser pulse initializes the NV center into the $|0\rangle$ spin state. Spin-dependent fluorescence from the NV spin states was detected using an avalanche photodiode. For each readout, we detected 0.088 and 0.06 photons from the $|0\rangle, |1\rangle$ states respectively. Before the experiments, the diamond was boiled in a 1:1:1 tri-acid mixture ($H_2SO_4$:$HNO_3$:$HClO_4$) for 4 hours at 180°C. The background magnetic noise at the frequencies detected here was determined to be at least 100 fold weaker than the measured signals, giving a measured NV coherence time of $> 1$ ms for decoupling performed at 500 kHz. A magnetic bias field of 360 G was used to lift the degeneracy of the $|-1\rangle, |+1\rangle$ spin states and create an effective qubit.

Using a 20 $\mu$m diameter copper wire placed on the diamond surface as an antenna, we applied microwave pulses resonant with the NV spin at 1.862 GHz, in addition to radio-frequency fields to be sensed at 500 kHz (with frequency detunings of up to 0.25 kHz). Resonant microwave pulses were generated with an Arbitrary Waveform Generator (Tektronix AWG70001A) and amplified to give a Rabi frequency of 36 MHz. Radio-frequency fields were generated with two independent signal generators (Rohde & Schwarz SMIQ03, Gigatronics 2520B), and combined with a coaxial RF-splitter used in reverse. Using an XY8-1 sequence centered at the generated RF frequency, we calibrated the amplitude of each RF signal at the NV center to be $460 \pm 20$ nT.

We used a Qdyne sensing sequence [3] to detect RF signals. The sequence consisted of a set of resonant pulses and waiting times according to $\pi/2 - [\tau/2 - \pi - \tau/2]^8 - \pi/2$, followed by a 500 ns laser pulse and a waiting time, where the first and last $\pi/2$ pulses had a relative 90° phase difference. The duration of $\tau + \pi$ was set to 1000 ns so that the NV center would be sensitive to fields fluctuating at 500 kHz. The waiting time was set to 1500 ns so that the recorded beat-note has a frequency equal to the signal detuning from 500 kHz. This sequence was run continuously for 0.25 seconds, and the number of photons detected for each of the 25,000 readouts was stored individually. The inset in Fig. 2a,2b shows a DFT of the photon timetrace. The analysis of this array of photon counts is plotted in Fig. 2 of the main text, where either a single frequency (detuning 251.6 Hz) or two frequencies (detuning 250 Hz and 251.6 Hz) from 500 kHz were applied. Statistical analysis was performed on 880 datasets obtained under identical experimental conditions.

## V. NANO NMR SIGNAL

Fig. 10 is a supplemental figure to Fig. 3 in the main text.


[1] Batalov, A., et al. "Temporal coherence of photons emitted by single nitrogen-vacancy defect centers in diamond using optical Rabi-oscillations." Phys. Rev. Lett. **100**, 077401 (2008).

[2] Liu, Shiyao, Huaiqing Wu, and William Q. Meeker. "Understanding and addressing the unbounded 'likelihood' problem." The American Statistician 69.3 : 191-200. (2015).

[3] Schmitt, Simon, et al. "Submillihertz magnetic spectroscopy performed with a nanoscale quantum sensor." Science 356.6340 (2017): 832-837.

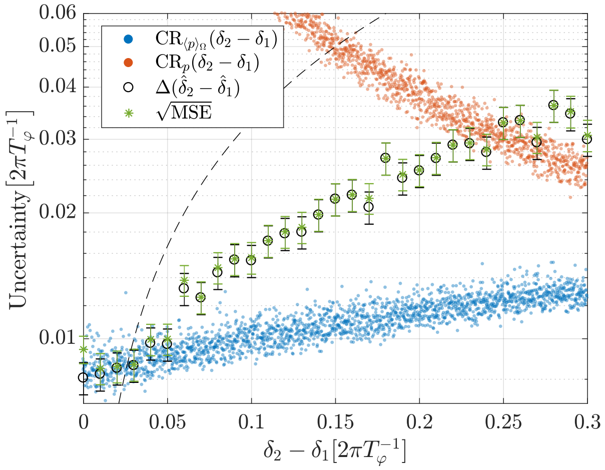


Figure 10. Same as Fig. 3 (in the main text) but with local search; i.e., initial estimations in the optimization process were the real values. The value of the likelihood function in this case was always larger than in the global search, which indicates that with more computing power the global search should converge to these results.
